# Supplementary material for: Mostly Harmless Simulations? Using Monte Carlo Studies for Estimator Selection
Source: arXiv:1809.09527 source file (2019-04-17)
Supplement: Supplementary file 1 [file appendix_stylisedsimulations.tex]

Here we provide further details on the parameters and procedures for the stylised simulations described in Subsection~\ref{subsec:AreScenarios2And3RelevantInTreatmentEffectEstimation} of \cite{AKS2019}.

%%%%%%%%%%%%%%%%%%
\subsection{Details of Simulations for Scenario~2}
%%%%%%%%%%%%%%%%%%

For each sample we generate 1,000 observations, and for each observation draw a covariate $x$ from a truncated standard normal distribution with the left truncation point at --4 and the right truncation point at 6.

Propensity score $e(x)$ is then constructed as 
\begin{equation}
	e(x) = .4 + .1 x.
	\label{eq:linearpsm}
\end{equation}
For each observation we draw a random number from a standard uniform distribution, and assign treated status, $D=1$, if $e(x)$ exceeds that random number.

We next generate an unobservable $\epsilon$ drawn from a normal distribution with mean zero. Since Scenario~2 is the heteroskedastic case, the standard deviation for those not treated is $\sigma_0 = .5$, while for those who are treated it is $\sigma_1 = 1.5$.\footnote{In the benchmark case (Scenario 1), mentioned at the end of Subsubsection~\ref{subsubsec:AnExampleForScenario2} in \cite{AKS2019}, $\sigma_0 = \sigma_1 = .5$.} 

Finally, the outcome $Y$ is generated as
\begin{equation}
	Y = 3 + .5 D + .5 X + \epsilon,
\end{equation}
and hence ATT is equal to .5.

This completes the generation of a Scenario~2 sample, which can then be used to implement the two EMCS procedures described in Section~\ref{sec:designs} of \cite{AKS2019}. For each EMCS design, we consider 1,000 samples and 1,000 replications per sample.

In the placebo design, we additionally require some choice of $\pi$ and $\lambda$, where $\lambda$ determines the degree of covariate overlap between the `placebo treated' and `placebo control' observations and $\pi$ determines the proportion of the `placebo treated'. We choose $\pi$ to ensure that the proportion of the `placebo treated' observations in each placebo EMCS replication is equal to the proportion of treated units in the sample. We follow \cite{HLW} in choosing $\lambda=1$. We also use a linear model to estimate the propensity score, as this corresponds to the true model in equation (\ref{eq:linearpsm}).

In the structured design, we first estimate the mean and variance of $X$ in a given sample, conditional on treatment status. We also regress $Y$ on $D$ and $X$, excluding the interaction of $D$ and $X$. Next, in the simulated dataset, $X$ is drawn from a normal distribution with mean and variance conditional on treatment status and equal to the estimates above. Whenever the draw of $X$ lies outside the support observed in the data, conditional on treatment status, the observation is replaced with the limit point of the support. Finally, the simulated outcome, $Y$, is generated in two steps. In the first step, we calculate its conditional mean based on the estimated coefficients from the regression above. In the second step, the simulated outcome is determined as a draw from a normal distribution with the conditional mean determined above and the variance that is equal to the variance of the residuals in the regression model estimated on the original data.\footnote{Thus, by using a single value of variance for both treated and control units, we fail to account for heteroskedasticity of the potential outcome equations. This is the source of misspecification of the structured design in Scenario~2.} Again, we replace extreme values with the limit of the support, conditional on treatment status.

We use two estimators in our stylised simulations: linear regression (OLS) and inverse probability weighting (IPW)\@. In the latter case, we first estimate the propensity score using a linear model, as this corresponds to the true model in equation (\ref{eq:linearpsm}), and then use inverse weighting with normalised weights to estimate the ATT\@.

%%%%%%%%%%%%%%%%%%
\subsection{Details of Simulations for Scenario~3}
%%%%%%%%%%%%%%%%%%

A similar procedure to that detailed in the previous subsection is followed. Two changes are made. First, we now have homoskedasticity so $\sigma_0 = \sigma_1 = .5$. Second, in each sample, we now generate the outcome $Y$ as
\begin{equation}
	Y = 3 + .5 D + .5 X + .5 X D + \epsilon,
\end{equation}
and hence ATT is equal to $.5 + .5 \cdot \E(X|D=1)$.\footnote{In practice, we estimate $\E(X|D=1)$ using the mean of $X$ for the treated observations in 1,000 samples from the true data generating process. As a result, ATT is equal to (approximately) .625.}

The source of misspecification of the structured design in Scenario~3 is in its failure to account for the interaction of $D$ and $X$ when generating the simulated outcomes.
\vfill
