# Supplementary material for: Mostly Harmless Simulations? Using Monte Carlo Studies for Estimator Selection
Source: arXiv:1809.09527 source file (2019-04-17)
Supplement: Supplementary file 2 [file appendix_stylisedtables.tex]

\vspace{2.5cm}

\begin{table}[htp]
  \centering
  \caption{\bf Simulation results for Scenario 1 in Section~\ref{sec:theory} of \cite{AKS2019}} \label{tab:tableA1}
  \begin{threeparttable}
  	\begin{tabular}{l >{\centering\arraybackslash}m{2.5cm} >{\centering\arraybackslash}m{2.5cm} >{\centering\arraybackslash}m{2.5cm}}
  	  \toprule
          & Absolute bias & RMSE  & SD \\
  	  \midrule
    \textbf{Original samples} &       &       &  \\
    IPW   & .000 & .034 & .034 \\
    OLS   & .000 & .032 & .032 \\
          &       &       &  \\
    \textbf{Placebo} &       &       &  \\
    IPW   & .002 & .044 & .044 \\
          & (.001) & (.002) & (.002) \\
    OLS   & .001 & .042 & .042 \\
          & (.001) & (.002) & (.002) \\
          &       &       &  \\
    \textbf{Structured} &       &       &  \\
    IPW   & .007 & .035 & .034 \\
          & (.005) & (.002) & (.001) \\
    OLS   & .001 & .033 & .033 \\
          & (.001) & (.001) & (.001) \\
  	  \bottomrule
  	\end{tabular}
  	\begin{footnotesize}
  	\begin{tablenotes}[flushleft]
    \item \textbf{Notes:} Results for `Original samples' correspond to the true values of all features of interest (absolute bias, RMSE, and SD) in the original data generating process. Measures of absolute bias and RMSE are centred around the true value of ATT, reported in Appendix~\ref{sec:appendix_stylisedsimulations}\@. All calculations are based on 1,000 samples.
For each of these 1,000 samples, `Placebo' and `Structured' generate 1,000 new replications using the placebo and structured approaches described in Section~\ref{sec:designs} of \cite{AKS2019}.
In each case, we report both the mean and the standard deviation (in brackets) of EMCS estimates of all features of interest across all replications. Estimates of absolute bias and RMSE are centred around 0 for placebo and around the model-implied value for structured.
For ease of interpretation, RMSE and SD are reported instead of MSE and variance (as elsewhere in the paper).
  	\end{tablenotes}
  	\end{footnotesize}
  \end{threeparttable}
\end{table}

\begin{table}[htp]
  \centering
  \caption{\bf Simulation results for Scenario 2 in Section~\ref{sec:theory} of \cite{AKS2019}} \label{tab:tableA2}
  \begin{threeparttable}
  	\begin{tabular}{l >{\centering\arraybackslash}m{2.5cm} >{\centering\arraybackslash}m{2.5cm} >{\centering\arraybackslash}m{2.5cm}}
  	  \toprule
          & Absolute bias & RMSE  & SD \\
  	  \midrule
    \textbf{Original samples} &       &       &  \\
    IPW   & .003 & .079 & .079 \\
    OLS   & .002 & .080 & .080 \\
          &       &       &  \\
    \textbf{Placebo} &       &       &  \\
    IPW   & .002 & .044 & .044 \\
          & (.001) & (.002) & (.002) \\
    OLS   & .001 & .042 & .042 \\
          & (.001) & (.002) & (.002) \\
          &       &       &  \\
    \textbf{Structured} &       &       &  \\
    IPW   & .016 & .070 & .067 \\
          & (.012) & (.005) & (.003) \\
    OLS   & .010 & .067 & .066 \\
          & (.008) & (.003) & (.003) \\
  	  \bottomrule
  	\end{tabular}
  	\begin{footnotesize}
  	\begin{tablenotes}[flushleft]
    \item \textbf{Notes:} Results for `Original samples' correspond to the true values of all features of interest (absolute bias, RMSE, and SD) in the original data generating process. Measures of absolute bias and RMSE are centred around the true value of ATT, reported in Appendix~\ref{sec:appendix_stylisedsimulations}\@. All calculations are based on 1,000 samples.
For each of these 1,000 samples, `Placebo' and `Structured' generate 1,000 new replications using the placebo and structured approaches described in Section~\ref{sec:designs} of \cite{AKS2019}.
In each case, we report both the mean and the standard deviation (in brackets) of EMCS estimates of all features of interest across all replications. Estimates of absolute bias and RMSE are centred around 0 for placebo and around the model-implied value for structured.
For ease of interpretation, RMSE and SD are reported instead of MSE and variance (as elsewhere in the paper).
  	\end{tablenotes}
  	\end{footnotesize}
  \end{threeparttable}
\end{table}

\begin{table}[htp]
  \centering
  \caption{\bf Simulation results for Scenario 3 in Section~\ref{sec:theory} of \cite{AKS2019}} \label{tab:tableA3}
  \begin{threeparttable}
  	\begin{tabular}{l >{\centering\arraybackslash}m{2.5cm} >{\centering\arraybackslash}m{2.5cm} >{\centering\arraybackslash}m{2.5cm}}
  	  \toprule
          & Absolute bias & RMSE  & SD \\
  	  \midrule
    \textbf{Original samples} &       &       &  \\
    IPW   & .001 & .044 & .044 \\
    OLS   & .081 & .089 & .037 \\
          &       &       &  \\
    \textbf{Placebo} &       &       &  \\
    IPW   & .002 & .043 & .043 \\
          & (.001) & (.002) & (.002) \\
    OLS   & .001 & .042 & .042 \\
          & (.001) & (.002) & (.002) \\
          &       &       &  \\
    \textbf{Structured} &       &       &  \\
    IPW   & .011 & .040 & .038 \\
          & (.009) & (.004) & (.001) \\
    OLS   & .003 & .037 & .036 \\
          & (.003) & (.001) & (.001) \\
  	  \bottomrule
  	\end{tabular}
  	\begin{footnotesize}
  	\begin{tablenotes}[flushleft]
    \item \textbf{Notes:} Results for `Original samples' correspond to the true values of all features of interest (absolute bias, RMSE, and SD) in the original data generating process. Measures of absolute bias and RMSE are centred around the true value of ATT, reported in Appendix~\ref{sec:appendix_stylisedsimulations}\@. All calculations are based on 1,000 samples.
For each of these 1,000 samples, `Placebo' and `Structured' generate 1,000 new replications using the placebo and structured approaches described in Section~\ref{sec:designs} of \cite{AKS2019}.
In each case, we report both the mean and the standard deviation (in brackets) of EMCS estimates of all features of interest across all replications. Estimates of absolute bias and RMSE are centred around 0 for placebo and around the model-implied value for structured.
For ease of interpretation, RMSE and SD are reported instead of MSE and variance (as elsewhere in the paper).
  	\end{tablenotes}
  	\end{footnotesize}
  \end{threeparttable}
\end{table}
