# Supplementary material for: Mostly Harmless Simulations? Using Monte Carlo Studies for Estimator Selection
Source: arXiv:1809.09527 source file (2019-04-17)
Supplement: Supplementary file 3 [file appendix_tables.tex]

\begin{table}[!h]
\begin{adjustwidth}{-1in}{-1in}
  \centering
  \caption{\bf Simulation results for Subsection~5.1 of \cite{AKS2019}} \label{tab:tableA4}
  \begin{threeparttable}
  	\begin{tabular}{l >{\centering\arraybackslash}m{4cm} >{\centering\arraybackslash}m{4cm} >{\centering\arraybackslash}m{4cm}}
  	  \toprule
          & Absolute bias & RMSE  & SD \\
  	  \midrule
    \textbf{Original samples} &       &       &  \\
    Doubly-robust regression & 142   & 1,019 & 1,010 \\
    IPW   & 51    & 1,102 & 1,101 \\
    Kernel matching & 818   & 1,382 & 1,115 \\
    OLS   & 306   & 740   & 674 \\
    Oaxaca--Blinder & 35    & 716   & 715 \\
    NN matching & 16    & 1,209 & 1,209 \\
    Bias-adjusted NN matching & 102   & 1,411 & 1,408 \\
          &       &       &  \\
    \textbf{Placebo} &       &       &  \\
    Doubly-robust regression & 280   & 1,817 & 1,785 \\
          & (206) & (236) & (234) \\
    IPW   & 323   & 1,960 & 1,928 \\
          & (161) & (225) & (221) \\
    Kernel matching & 68    & 1,244 & 1,242 \\
          & (50)  & (141) & (139) \\
    OLS   & 385   & 901   & 776 \\
          & (287) & (152) & (37) \\
    Oaxaca--Blinder & 420   & 927   & 783 \\
          & (311) & (171) & (40) \\
    NN matching & 241   & 2,423 & 2,407 \\
          & (172) & (326) & (318) \\
    Bias-adjusted NN matching & 319   & 3,531 & 3,509 \\
          & (392) & (11,085) & (11,086) \\
  	  \bottomrule
  	\end{tabular}
  	\begin{footnotesize}
  	\begin{tablenotes}[flushleft]
    \item \textbf{Notes:} Results for `Original samples' correspond to the true values of all features of interest (absolute bias, RMSE, and SD) in the original data generating process. Measures of absolute bias and RMSE are centred around the true value of ATT, equal to \$1,794. All calculations are based on 1,000 samples.
For each of these 1,000 samples, `Placebo' and `Structured' generate 1,000 new replications using the placebo and structured approaches described in Section~\ref{sec:designs} of \cite{AKS2019}. Similarly, `Bootstrap' generates 1,000 nonparametric bootstrap replications by sampling with replacement the same number of observations as the original data.
In each of the three cases, we report both the mean and the standard deviation (in brackets) of EMCS estimates of all features of interest across all replications. Estimates of absolute bias and RMSE are centred around 0 for placebo, around the model-implied value for structured, and around the point estimate in the original sample for bootstrap. 
For ease of interpretation, RMSE and SD are reported instead of MSE and variance (as in Table~\ref{tab:table1} in \cite{AKS2019}). The `minimum' value for each feature, as reported in Table~\ref{tab:table1} in \cite{AKS2019}, is its lowest value among our estimators in the original data generating process (\textit{i.e.}~the lowest value in the `Original samples' panel). The minimum value of absolute bias is 16; for MSE, it is 512,322 (or $\simeq$716$^2$); for variance, it is 454,278 (or $\simeq$674$^2$).
  	\end{tablenotes}
  	\end{footnotesize}
  \end{threeparttable}
\end{adjustwidth}
\end{table}

\setcounter{table}{0}

\begin{table}[htp]
\begin{adjustwidth}{-1in}{-1in}
  \centering
  \caption{\bf Simulation results for Subsection~5.1 of \cite{AKS2019} (cont.)} \label{tab:tableA5}
  \begin{threeparttable}
  	\begin{tabular}{l >{\centering\arraybackslash}m{4cm} >{\centering\arraybackslash}m{4cm} >{\centering\arraybackslash}m{4cm}}
  	  \toprule
          & Absolute bias & RMSE  & SD \\
  	  \midrule
    \textbf{Structured} &       &       &  \\
    Doubly-robust regression & 620   & 1,402 & 1,261 \\
          & (492) & (340) & (113) \\
    IPW   & 591   & 1,436 & 1,310 \\
          & (488) & (331) & (124) \\
    Kernel matching & 408   & 1,458 & 1,426 \\
          & (371) & (254) & (145) \\
    OLS   & 558   & 1,125 & 1,006 \\
          & (476) & (359) & (105) \\
    Oaxaca--Blinder & 690   & 1,192 & 997 \\
          & (495) & (389) & (103) \\
    NN matching & 626   & 1,660 & 1,533 \\
          & (492) & (311) & (122) \\
    Bias-adjusted NN matching & 620   & 1,634 & 1,509 \\
          & (491) & (312) & (119) \\
          &       &       &  \\
    \textbf{Bootstrap} &       &       &  \\
    Doubly-robust regression & 128 & 1,197 & 1,186 \\
          & (122) & (203) & (193) \\
    IPW   &  86 & 1,305 & 1,301 \\
          & (84) & (235) & (231) \\
    Kernel matching & 652 & 1,789 & 1,610 \\
          & (495) & (307) & (189) \\
    OLS   &  24 & 906   & 906 \\
          & (18) & (68)  & (68) \\
    Oaxaca--Blinder &  25 & 961   & 961 \\
          & (19) & (93)  & (93) \\
    NN matching & 552 & 1,653 & 1,518 \\
          & (414) & (325) & (250) \\
    Bias-adjusted NN matching & 703 & 3,126 & 2,980 \\
          & (637) & (3,560) & (3,562) \\
  	  \bottomrule
  	\end{tabular}
  	\begin{footnotesize}
  	\begin{tablenotes}[flushleft]
    \item \textbf{Notes:} Results for `Original samples' correspond to the true values of all features of interest (absolute bias, RMSE, and SD) in the original data generating process. Measures of absolute bias and RMSE are centred around the true value of ATT, equal to \$1,794. All calculations are based on 1,000 samples.
For each of these 1,000 samples, `Placebo' and `Structured' generate 1,000 new replications using the placebo and structured approaches described in Section~\ref{sec:designs} of \cite{AKS2019}. Similarly, `Bootstrap' generates 1,000 nonparametric bootstrap replications by sampling with replacement the same number of observations as the original data.
In each of the three cases, we report both the mean and the standard deviation (in brackets) of EMCS estimates of all features of interest across all replications. Estimates of absolute bias and RMSE are centred around 0 for placebo, around the model-implied value for structured, and around the point estimate in the original sample for bootstrap. 
For ease of interpretation, RMSE and SD are reported instead of MSE and variance (as in Table~\ref{tab:table1} in \cite{AKS2019}). The `minimum' value for each feature, as reported in Table~\ref{tab:table1} in \cite{AKS2019}, is its lowest value among our estimators in the original data generating process (\textit{i.e.}~the lowest value in the `Original samples' panel). The minimum value of absolute bias is 16; for MSE, it is 512,322 (or $\simeq$716$^2$); for variance, it is 454,278 (or $\simeq$674$^2$).
  	\end{tablenotes}
  	\end{footnotesize}
  \end{threeparttable}
\end{adjustwidth}
\end{table}

\begin{table}[htp]
\begin{adjustwidth}{-1in}{-1in}
  \centering
  \caption{\bf Simulation results for Subsection~5.2 of \cite{AKS2019}} \label{tab:tableA6}
  \begin{threeparttable}
  	\begin{tabular}{l >{\centering\arraybackslash}m{4cm} >{\centering\arraybackslash}m{4cm} >{\centering\arraybackslash}m{4cm}}
  	  \toprule
          & Absolute bias & RMSE  & SD \\
  	  \midrule
    \textbf{Original samples} &       &       &  \\
    Doubly-robust regression & 1,222 & 1,566 & 980 \\
    IPW   & 1,081 & 1,514 & 1,060 \\
    Kernel matching & 1,356 & 1,652 & 944 \\
    OLS   & 1,111 & 1,237 & 545 \\
    Oaxaca--Blinder & 954   & 1,106 & 559 \\
    NN matching & 1,122 & 1,732 & 1,320 \\
    Bias-adjusted NN matching & 1,101 & 1,847 & 1,484 \\
          &       &       &  \\
    \textbf{Placebo} &       &       &  \\
    Doubly-robust regression & 263   & 1,823 & 1,794 \\
          & (196) & (198) & (197) \\
    IPW   & 203   & 2,026 & 2,013 \\
          & (132) & (197) & (198) \\
    Kernel matching & 78    & 1,487 & 1,483 \\
          & (88)  & (267) & (263) \\
    OLS   & 379   & 909   & 791 \\
          & (284) & (153) & (36) \\
    Oaxaca--Blinder & 408   & 930   & 797 \\
          & (304) & (171) & (37) \\
    NN matching & 219   & 2,480 & 2,467 \\
          & (156) & (253) & (250) \\
    Bias-adjusted NN matching & 290   & 3,233 & 3,214 \\
          & (226) & (1,852) & (1,853) \\
  	  \bottomrule
  	\end{tabular}
  	\begin{footnotesize}
  	\begin{tablenotes}[flushleft]
    \item \textbf{Notes:} Results for `Original samples' correspond to the true values of all features of interest (absolute bias, RMSE, and SD) in the original data generating process. Measures of absolute bias and RMSE are centred around the true value of ATT, equal to \$0. All calculations are based on 1,000 samples.
For each of these 1,000 samples, `Placebo' and `Structured' generate 1,000 new replications using the placebo and structured approaches described in Section~\ref{sec:designs} of \cite{AKS2019}. Similarly, `Bootstrap' generates 1,000 nonparametric bootstrap replications by sampling with replacement the same number of observations as the original data.
In each of the three cases, we report both the mean and the standard deviation (in brackets) of EMCS estimates of all features of interest across all replications. Estimates of absolute bias and RMSE are centred around 0 for placebo, around the model-implied value for structured, and around the point estimate in the original sample for bootstrap. 
For ease of interpretation, RMSE and SD are reported instead of MSE and variance (as in Table~\ref{tab:table2} in \cite{AKS2019}). The `minimum' value for each feature, as reported in Table~\ref{tab:table2} in \cite{AKS2019}, is its lowest value among our estimators in the original data generating process (\textit{i.e.}~the lowest value in the `Original samples' panel). The minimum value of absolute bias is 954; for MSE, it is 1,222,627 (or $\simeq$1,106$^2$); for variance, it is 296,671 (or $\simeq$545$^2$).
  	\end{tablenotes}
  	\end{footnotesize}
  \end{threeparttable}
\end{adjustwidth}
\end{table}

\setcounter{table}{1}

\begin{table}[htp]
\begin{adjustwidth}{-1in}{-1in}
  \centering
  \caption{\bf Simulation results for Subsection~5.2 of \cite{AKS2019} (cont.)} \label{tab:tableA7}
  \begin{threeparttable}
  	\begin{tabular}{l >{\centering\arraybackslash}m{4cm} >{\centering\arraybackslash}m{4cm} >{\centering\arraybackslash}m{4cm}}
  	  \toprule
          & Absolute bias & RMSE  & SD \\
  	  \midrule
    \textbf{Structured} &       &       &  \\
    Doubly-robust regression & 1,009 & 1,440 & 1,065 \\
          & (398) & (327) & (70) \\
    IPW   & 1,027 & 1,500 & 1,120 \\
          & (401) & (326) & (84) \\
    Kernel matching & 827   & 1,411 & 1,156 \\
          & (405) & (301) & (86) \\
    OLS   & 1,023 & 1,295 & 858 \\
          & (395) & (351) & (60) \\
    Oaxaca--Blinder & 1,072 & 1,327 & 851 \\
          & (389) & (351) & (57) \\
    NN matching & 1,041 & 1,704 & 1,364 \\
          & (403) & (303) & (84) \\
    Bias-adjusted NN matching & 1,010 & 1,642 & 1,318 \\
          & (398) & (301) & (76) \\
          &       &       &  \\
    \textbf{Bootstrap} &       &       &  \\
    Doubly-robust regression & 155 & 1,152 & 1,136 \\
          & (127) & (189) & (180) \\
    IPW   &  84 & 1,262 & 1,258 \\
          & (77) & (233) & (231) \\
    Kernel matching & 430 & 1,452 & 1,352 \\
          & (369) & (284) & (208) \\
    OLS   &  23 & 849   & 849 \\
          & (17) & (45)  & (44) \\
    Oaxaca--Blinder & 21 & 853   & 853 \\
          & (16) & (43)  & (43) \\
    NN matching & 643 & 1,789 & 1,615 \\
          & (530) & (450) & (321) \\
    Bias-adjusted NN matching & 839 & 3,356 & 3,180 \\
          & (804) & (1,025) & (932) \\
  	  \bottomrule
  	\end{tabular}
  	\begin{footnotesize}
  	\begin{tablenotes}[flushleft]
    \item \textbf{Notes:} Results for `Original samples' correspond to the true values of all features of interest (absolute bias, RMSE, and SD) in the original data generating process. Measures of absolute bias and RMSE are centred around the true value of ATT, equal to \$0. All calculations are based on 1,000 samples.
For each of these 1,000 samples, `Placebo' and `Structured' generate 1,000 new replications using the placebo and structured approaches described in Section~\ref{sec:designs} of \cite{AKS2019}. Similarly, `Bootstrap' generates 1,000 nonparametric bootstrap replications by sampling with replacement the same number of observations as the original data.
In each of the three cases, we report both the mean and the standard deviation (in brackets) of EMCS estimates of all features of interest across all replications. Estimates of absolute bias and RMSE are centred around 0 for placebo, around the model-implied value for structured, and around the point estimate in the original sample for bootstrap. 
For ease of interpretation, RMSE and SD are reported instead of MSE and variance (as in Table~\ref{tab:table2} in \cite{AKS2019}). The `minimum' value for each feature, as reported in Table~\ref{tab:table2} in \cite{AKS2019}, is its lowest value among our estimators in the original data generating process (\textit{i.e.}~the lowest value in the `Original samples' panel). The minimum value of absolute bias is 954; for MSE, it is 1,222,627 (or $\simeq$1,106$^2$); for variance, it is 296,671 (or $\simeq$545$^2$).
  	\end{tablenotes}
  	\end{footnotesize}
  \end{threeparttable}
\end{adjustwidth}
\end{table}

\begin{table}[htp]
\begin{adjustwidth}{-1in}{-1in}
  \centering
  \caption{\bf Simulation results for Subsection~5.3 of \cite{AKS2019}} \label{tab:tableA8}
  \begin{threeparttable}
  	\begin{tabular}{l >{\centering\arraybackslash}m{4cm} >{\centering\arraybackslash}m{4cm} >{\centering\arraybackslash}m{4cm}}
  	  \toprule
          & Absolute bias & RMSE  & SD \\
  	  \midrule
    \textbf{Original samples} &       &       &  \\
    Doubly-robust regression & 68    & 1,573 & 1,572 \\
    IPW   & 565   & 1,682 & 1,585 \\
    Kernel matching & 540   & 1,649 & 1,559 \\
    OLS   & 1,069 & 1,131 & 371 \\
    Oaxaca--Blinder & 171   & 583   & 558 \\
    NN matching & 442   & 2,374 & 2,333 \\
    Bias-adjusted NN matching & 102   & 1,837 & 1,835 \\
          &       &       &  \\
    \textbf{Placebo} &       &       &  \\
    Doubly-robust regression & 174   & 1,721 & 1,709 \\
          & (134) & (156) & (153) \\
    IPW   & 187   & 2,162 & 2,153 \\
          & (117) & (172) & (171) \\
    Kernel matching & 144   & 1,925 & 1,917 \\
          & (140) & (281) & (277) \\
    OLS   & 208   & 651   & 600 \\
          & (160) & (72)  & (26) \\
    Oaxaca--Blinder & 298   & 753   & 664 \\
          & (224) & (116) & (30) \\
    NN matching & 175   & 2,705 & 2,699 \\
          & (136) & (242) & (238) \\
    Bias-adjusted NN matching & 175   & 1,942 & 1,931 \\
          & (137) & (174) & (171) \\
  	  \bottomrule
  	\end{tabular}
  	\begin{footnotesize}
  	\begin{tablenotes}[flushleft]
    \item \textbf{Notes:} Results for `Original samples' correspond to the true values of all features of interest (absolute bias, RMSE, and SD) in the original data generating process. Measures of absolute bias and RMSE are centred around the true value of ATT, equal to --\$405. All calculations are based on 1,000 samples.
For each of these 1,000 samples, `Placebo' and `Structured' generate 500 new replications using the placebo and structured approaches described in Section~\ref{sec:designs} of \cite{AKS2019}. Similarly, `Bootstrap' generates 500 nonparametric bootstrap replications by sampling with replacement the same number of observations as the original data.
In each of the three cases, we report both the mean and the standard deviation (in brackets) of EMCS estimates of all features of interest across all replications. Estimates of absolute bias and RMSE are centred around 0 for placebo, around the model-implied value for structured, and around the point estimate in the original sample for bootstrap. 
For ease of interpretation, RMSE and SD are reported instead of MSE and variance (as in Table~\ref{tab:table3} in \cite{AKS2019}). The `minimum' value for each feature, as reported in Table~\ref{tab:table3} in \cite{AKS2019}, is its lowest value among our estimators in the original data generating process (\textit{i.e.}~the lowest value in the `Original samples' panel). The minimum value of absolute bias is 68; for MSE, it is 340,300 (or $\simeq$583$^2$); for variance, it is 137,574 (or $\simeq$371$^2$).
  	\end{tablenotes}
  	\end{footnotesize}
  \end{threeparttable}
\end{adjustwidth}
\end{table}

\setcounter{table}{2}

\begin{table}[htp]
\begin{adjustwidth}{-1in}{-1in}
  \centering
  \caption{\bf Simulation results for Subsection~5.3 of \cite{AKS2019} (cont.)} \label{tab:tableA9}
  \begin{threeparttable}
  	\begin{tabular}{l >{\centering\arraybackslash}m{4cm} >{\centering\arraybackslash}m{4cm} >{\centering\arraybackslash}m{4cm}}
  	  \toprule
          & Absolute bias & RMSE  & SD \\
  	  \midrule
    \textbf{Structured} &       &       &  \\
    Doubly-robust regression & 198   & 819   & 816 \\
          & (116) & (78)  & (65) \\
    IPW   & 194   & 1,228 & 1,224 \\
          & (121) & (119) & (116) \\
    Kernel matching & 149   & 910   & 913 \\
          & (116) & (107) & (106) \\
    OLS   & 405   & 631   & 470 \\
          & (253) & (172) & (20) \\
    Oaxaca--Blinder & 202   & 509   & 503 \\
          & (114) & (54)  & (21) \\
    NN matching & 140   & 1,205 & 1,210 \\
          & (107) & (113) & (111) \\
    Bias-adjusted NN matching & 200   & 942   & 939 \\
          & (117) & (81)  & (71) \\
          &       &       &  \\
    \textbf{Bootstrap} &       &       &  \\
    Doubly-robust regression & 283 & 1,347 & 1,304 \\
          & (252) & (396) & (363) \\
    IPW   & 159 & 1,177 & 1,157 \\
          & (303) & (625) & (570) \\
    Kernel matching & 381 & 1,276 & 1,187 \\
          & (365) & (512) & (456) \\
    OLS   &  15 & 415   & 415 \\
          & (12) & (23)  & (23) \\
    Oaxaca--Blinder & 22 & 620   & 620 \\
          & (17) & (33)  & (33) \\
    NN matching & 953 & 2,245 & 1,974 \\
          & (808) & (967) & (726) \\
    Bias-adjusted NN matching & 689 & 1,946 & 1,763 \\
          & (574) & (555) & (435) \\
  	  \bottomrule
  	\end{tabular}
  	\begin{footnotesize}
  	\begin{tablenotes}[flushleft]
    \item \textbf{Notes:} Results for `Original samples' correspond to the true values of all features of interest (absolute bias, RMSE, and SD) in the original data generating process. Measures of absolute bias and RMSE are centred around the true value of ATT, equal to --\$405. All calculations are based on 1,000 samples.
For each of these 1,000 samples, `Placebo' and `Structured' generate 500 new replications using the placebo and structured approaches described in Section~\ref{sec:designs} of \cite{AKS2019}. Similarly, `Bootstrap' generates 500 nonparametric bootstrap replications by sampling with replacement the same number of observations as the original data.
In each of the three cases, we report both the mean and the standard deviation (in brackets) of EMCS estimates of all features of interest across all replications. Estimates of absolute bias and RMSE are centred around 0 for placebo, around the model-implied value for structured, and around the point estimate in the original sample for bootstrap. 
For ease of interpretation, RMSE and SD are reported instead of MSE and variance (as in Table~\ref{tab:table3} in \cite{AKS2019}). The `minimum' value for each feature, as reported in Table~\ref{tab:table3} in \cite{AKS2019}, is its lowest value among our estimators in the original data generating process (\textit{i.e.}~the lowest value in the `Original samples' panel). The minimum value of absolute bias is 68; for MSE, it is 340,300 (or $\simeq$583$^2$); for variance, it is 137,574 (or $\simeq$371$^2$).
  	\end{tablenotes}
  	\end{footnotesize}
  \end{threeparttable}
\end{adjustwidth}
\end{table}
